# Supplementary material for: psPRF:Pansharpening Planar Neural Radiance Field for Generalized 3D Reconstruction Satellite Imagery
Source: arXiv:2406.15707 source file (2024-06-22)
Supplement: Supplementary file 1 [file appendix.tex]

\subsection{Compare with MVS}
\label{sec:comp_mvs}
% \subsection{Comparison with state-of-the-art methods on Pansharpening}
\paragraph{dataset}
\paragraph{comparison}
\paragraph{result}

\subsection{Efficiency}
\label{sec:exp_efficiency}
In addition to image quality evaluation,  we also compare the models by memory and computation consumption, time cost, and the model parameters. 
rpcPRF-single and rpcPRF-sparse, despite their differences in inputs and training processes, share identical memory and computation consumption at inference time.
Notably,  rpcPRF-single and rpcPRF-sparse, despite their differences in inputs and training processes, share identical memory and computation consumption at inference time.  The three models are presented for comparison in Table~\ref{tab:comp_nerf_memory}.  

The two metrics \textbf{FLOPs} and \textbf{Time} are calculated for a triple of images. NeRF-based models are rendered per ray, so the temporary memory depends on the batch size of rays, while rpcPRF series rendered per image, so we set the batch size of S-NeRF and Sat-NeRF to be $3 \times H \times W$.
Table~\ref{tab:comp_nerf_memory} shows that the proposed rpcPRF has nearly 20x faster inference speed than Sat-NeRF. 
Besides, for most of the current single-GPU settings, the batch size of $3\times H\times W$ rays is unattainable, so the total inference time of rpcPRF is far less than NeRF-based models.
\begin{table}
    \centering
     \caption{Time and computation comparisons of NeRF-based methods and the proposed rpcPRF-single and rpcPRF-sparse}
      \label{tab:comp_nerf_memory}
      %\resizebox{8cm}{!}{
    \begin{tabular}{c|cccc}
    \toprule
        sites & \textbf{Memory}$\downarrow$ & \textbf{Param}$\downarrow$& \textbf{FLOPs}$\downarrow$& \textbf{Time}$\downarrow$\\
        \midrule
EO-NeRF&2.863G & \textbf{0.63M}& 103.08G& 23.295s \\
Sat-NeRF&3.147G &0.66M &338.43G & 24.263s\\
rpcPRF-single(sparse)& \textbf{0.477G}&19.79M&\textbf{202.23G} & \textbf{0.954s}\\
         \bottomrule
    \end{tabular}
    \vspace{-0.5cm}
\end{table}

% \subsection{Single-view rpcPRF and ablation study}

\subsection{Ablation Study}
To investigate the effectiveness of various components in psPRF,
we conducted the following experiments on WorldView3 dataset with stereo settings.
\subsubsection{Study on the reprojection loss}
report the results in Table~\ref{tab:ablation_reprojection}

\subsubsection{Study on the depth map supervision}
With the setting of a radiance field, the 3D reconstruction is conducted in a unsupervised way.

\begin{table*}
  \centering  
    \caption{Source view synthesis comparison on HR-PAN, LR-RGB pairs over different scenes.}  
  \fontsize{4}{4}\selectfont
  % \LARGE
  \resizebox{16cm}{!}{
  \begin{threeparttable}  
    %\resizebox{16cm}{!}{
    \begin{tabular}{ccccccc}  
    \toprule  
    %\multirow{2}{*}{Dataset}  
    &\multicolumn{2}{c}{\textbf{PSNR}$\uparrow$}&\multicolumn{2}{c}{\textbf{SSIM}$\uparrow$}&\multicolumn{2}{c}{\textbf{LPIPS}$\downarrow$}\cr  
    \cmidrule(lr){2-3} \cmidrule(lr){4-5}\cmidrule(lr){6-7}  
    Sites&rpcPRF&psPRF&rpcPRF&psPRF&rpcPRF&psPRF\cr 
    \midrule  
 \\
    \bottomrule  
    \end{tabular}  
   % }
    \end{threeparttable}
    }
    \label{tab:comp_across_scene_ps}
\end{table*}
\begin{table*}
  \centering  
    \caption{Novel view synthesis comparison on HR-PAN, LR-RGB pairs over different scenes.}  
  \fontsize{4}{4}\selectfont
  % \LARGE
  \resizebox{16cm}{!}{
  \begin{threeparttable}  
    %\resizebox{16cm}{!}{
    \begin{tabular}{ccccccc}  
    \toprule  
    %\multirow{2}{*}{Dataset}  
    &\multicolumn{2}{c}{\textbf{PSNR}$\uparrow$}&\multicolumn{2}{c}{\textbf{SSIM}$\uparrow$}&\multicolumn{2}{c}{\textbf{LPIPS}$\downarrow$}\cr  
    \cmidrule(lr){2-3} \cmidrule(lr){4-5}\cmidrule(lr){6-7}  
    Sites&rpcPRF&psPRF&rpcPRF&psPRF&rpcPRF&psPRF\cr 
    \midrule  
 \\
    \bottomrule  
    \end{tabular}  
   % }
    \end{threeparttable}
    }
    \label{tab:comp_across_scene}
\end{table*}
